# Supplementary material for: Logic Query of Thoughts: Guiding Large Language Models to Answer Complex Logic Queries with Knowledge Graphs
Source: arXiv:2404.04264 source file (2024-12-12)
Supplement: Supplementary file 1 [file 100supplement.tex]

%\hh{lihui: i hid some results to meet 2-page limit (1) check the text/figure/table to see if they are consistent; (2) check if the results here are consistent with what we said in 9-page content (e.g., we say 'xxxx results can be found in appendix there, but here we might have hidden them; (3) why are there two empty pages at the end?}
\vspace{-0.3\baselineskip}
\subsection{A -- Predicate Entropy and Similarity Examples}
\vspace{-0.3\baselineskip}
Here, we use Figure ~\ref{inconsistency} to give two examples on how to calculate the predicate entropy and predicate-predicate similarity. 
For the predicate entropy, 
suppose we want to calculate the entropy for {\tt command}. Three entities ({\tt President}, {\tt US Army} and {\tt Air Force}) have {\tt command} as their out links, and the numbers of out links of {\tt command} are 2, 3 and 2, respectively. 
Therefore, 
$V_i^2 = \{{\tt President}, {\tt Air Force} \}$, $V_i^3 = \{ {\tt US Army} \}$ and $V_i^d = \emptyset$ otherwise. Therefore, we have 
$E({\tt command}) = -\frac{2}{3} \log(\frac{2}{3}) - \frac{1}{3}\log(\frac{1}{3}) = 0.92$ and $w({\tt command}) = 0.43$.

For the predicate-predicate similarity,
suppose we want to calculate the similarity between {\tt major} and {\tt study}. Both {\tt major} and {\tt study}  have only one adjacent neighboring predicate {\tt graduate}. This means that for any predicate $i \neq {\tt graduate}$, $U({\tt major}, i) = U({\tt study}, i) = 0$.
Since $\textrm{E}({\tt graduate}) = 0$, we have ${w}({\tt graduate}) = 2\sigma(\infty) - 1 = 1$. We have \textrm{TF}({\tt major}, {\tt graduate}) = \textrm{TF}({\tt study}, {\tt graduate}) = $\log(1 + 1 \times 1) = 1$, and $U({\tt major}, {\tt graduate}) = U({\tt study}, {\tt graduate}) = IDF({\tt graduate}) = \log\frac{8}{4} = 1$. If we compare the two vectors, $U_{{\tt major}}$ and $U_{{\tt study}}$, we find that they are the same. Therefore, we have that $\textrm{Sim}({\tt major}, {\tt study}) = 1$.

\vspace{-0.8\baselineskip}
\subsection{B -- Proof of Lemma ~\ref{lm:collectiveinfluence}}

\begin{proof}
We rewrite the loss function as 
\setlength{\abovedisplayskip}{1pt}
\setlength{\belowdisplayskip}{1pt}
\begin{small}
\[
Loss = || H_1 - H_2 ||_F^2 = \sum_{i,j} (h_{e_{i,j}} - h_{c_{i,j}})^2
\vspace{-0.6\baselineskip}
\]
Take the derivative, together with Lemma 1, we have 
\begin{equation}
\begin{aligned}    
I(A_n(i,j)) &= \sum_{k \in N(n)} -2(h_{e_{k,n}} - h_{c_{k,n}})\frac{\partial sim(KS_n, KS_k)}{\partial A_n(i,j)} \\
\vspace{-0.6\baselineskip}
(N_n(i)) &= \sum_{k \in N(n)} -2(h_{e_{k,n}} - h_{c_{k,n}})\frac{\partial sim(KS_n, KS_k)}{\partial N_n(i)}  \\
I(N_n^l(i,i)) &= \sum_{k \in N(n)} -2(h_{e_{k,n}} - h_{c_{k,n}})\frac{\partial sim(KS_n, KS_k)}{\partial N_n^l(i,i)}
\end{aligned}
\end{equation}
\end{small}
which completes the proof.
\end{proof}

\vspace{-0.8\baselineskip}
\subsection{C -- Node-specific Knowledge Segments Results}

Figure ~\ref{nibble-hawaii} shows another node-specific knowledge segment w.r.t. the query node {\tt Hawaii}. We can see 
many landmarks in {\tt Hawaii}, e.g. ,{\tt Hawaii Convention Center}, {\tt Hawaii State Capitol}, {\tt Aloha Stadium}. We also find that {\tt Honolulu} is the capital of {\tt Hawaii}.

\begin{figure}[ht]
\vspace{-0.6\baselineskip}
	\centering
	\includegraphics[width=0.35\textwidth, height=0.16\textwidth]{img/nibble-hawaii.png}
	\vspace{-1\baselineskip}
	\caption{Node-specific knowledge segment of {\tt Hawaii}.}
	\label{nibble-hawaii}
	\vspace{-0.8\baselineskip}
\end{figure}

{
\vspace{-0.8\baselineskip}
\FloatBarrier
\subsection{D -- Predicate Similarity Results}
Table ~\ref{appendix-pred-sim} shows the predicate similarity between {\tt isTypeOf} and other predicates. %We only list the predicates we used in this paper.
\begin{table}[!htbp]
    \centering
    \vspace{-0.8\baselineskip}
    \scriptsize
    \caption{Predicate similarity of {\tt isTypeOf} with others}
    \vspace{-2\baselineskip}
    \begin{tabular}{ |c|c|c|c|c|c|c|c| }
  \hline
  predicate & sim & predicate & sim & predicate & sim & predicate & sim \\
  \hline
 isCitizenOf &  0.840 &  isLeaderOf &  0.955 & isAffiliatedTo &  0.808 &  isPoliticianOf &  0.917 \\
 livesIn &  0.972 &  owns &  0.945 & exports &  0.706 &  dealsWith &  0.697\\
 hasCapital &  0.786 &  command &  0.216 & happenedIn &  0.767 &  participatedIn &  0.869\\
 worksAt &  0.752 &  isLocatedIn &  0.870 & & & &\\
  \hline
\end{tabular}
\label{appendix-pred-sim}
\end{table}
}

\FloatBarrier
\subsection{E -- Influence Function Results}

Table ~\ref{iraq_pair-node-attr} and Table ~\ref{iraq_pair-edge1} show the node attribute/node influence value and edge influence value of the pair-wise comparative reasoning example we used in section ~\ref{exp-pair-section}.
\begin{table}[ht]
\vspace{-1\baselineskip}
\caption{Pairwise node attribute influence ranking}
\vspace{-1\baselineskip}
\scriptsize
\subfloat[Node attribute influence: $KS_1$]
{\begin{tabular}{|c|c|c|}
\hline
 Rank & Predicate & value \\
\hline
1 & Washington, D.C & 4.49 $e^{-5}$\\
2 & United States President &  3.92 $e^{-5}$  \\
3 & White House & 3.90$e^{-5}$   \\
4 & United States & 3.87$e^{-5}$    \\
5 & United States Army  & 1.96$e^{-5}$    \\
6 & Afghanistan & 1.95$e^{-5}$    \\
7 & Operation Mountain Thrust   &  1.95$e^{-5}$  \\
\hline
\end{tabular}}
%\vspace*{0.1cm}
\subfloat[Node attribute influence: $KS_2$]{
\begin{tabular}{|c|c|c|}
\hline
Rank & Predicate & value \\
\hline
1 & Washington, D.C & 4.51$e^{-5}$    \\
2 & White House   &  3.90$e^{-5}$  \\
3 & United States  & 3.87$e^{-5}$    \\
4 & United States President &  3.83$e^{-5}$  \\
5 & Iraq & 1.97$e^{-5}$    \\
6 & Iraqi Army & 1.86$e^{-5}$   \\
\hline
\end{tabular}}
\\
\vspace{-1.0\baselineskip}
\subfloat[Node influence: $KS_1$]
{\begin{tabular}{|c|c|c|}
\hline
Rank & Predicate & value \\
\hline
1 & Washington, D.C   &  1.54$e^{-5}$  \\
2 & United States President & 6.88 $e^{-6}$\\
3 & United States & 6.18$e^{-6}$    \\
4 & White House & 5.37$e^{-6}$   \\
5 & United States Army  & 3.06$e^{-6}$    \\
6 & Operation Mountain Thrust &  3.06 $e^{-6}$  \\
7 & Afghanistan & 3.06$e^{-6}$    \\
\hline
\end{tabular}}
%\vspace*{2cm}
\subfloat[Node influence: $KS_2$]
{
\begin{tabular}{|c|c|c|}
\hline
Rank & Predicate & value \\
\hline
1 & Washington, D.C   &   1.47$e^{-5}$ \\
2 & United States      &   6.19$e^{-6}$ \\
3 & White House  & 5.37$e^{-6}$      \\
4 & United States President & 4.66$e^{-6}$     \\
5 & Iraq    &    3.04$e^{-6}$      \\
6 & Iraqi Army    &   1.50$e^{-6}$      \\
\hline
\end{tabular}}
\label{iraq_pair-node-attr}
\vspace{-2\baselineskip}
\end{table}
\begin{table}[ht]
    \centering
    \scriptsize
    \vspace{-2\baselineskip}
    \caption{Pairwise edge influence ranking}
    \vspace{-1\baselineskip}
    \begin{tabular}{ |c|c|c| }
\hline
\multicolumn{3}{|c|}{Edge influence of $KS_1$} \\\hline
  Rank & Triple & value \\
  \hline
  1 & <United States President, livesIn, Washington, D.C> & 4.28$e^{-4}$ \\
  2 & <United States, hasCapital, Washington, D.C> & 4.28 $e^{-4}$ \\
  3 & <United States President, isLeaderOf, US Army> & 3.67$e^{-4}$ \\
  4 & <United States, dealsWith, Afghanistan> &  3.67 $e^{-4}$ \\
  5 & <White House, isLocatedIn, Washington, D.C> & 3.59 $e^{-4}$ \\
  6 & <Afghanistan, participatedIn, Operation Mountain Thrust> & 3.59 $e^{-4}$ \\
  7 & <US Army, participatedIn, Operation Mountain Thrust> & 3.59$e^{-4}$ \\
  \hline
  \multicolumn{3}{|c|}{Edge influence of $KS_2$} \\\hline
  Rank & Triple & value \\
  \hline
  1 & <United States, hasCapital, Washington, D.C> & 4.51 $e^{-4}$ \\
  2 & <United States, dealsWith, Iraq> &  3.89 $e^{-4}$ \\
  3 & <White House, isLocatedIn, Washington, D.C> & 3.83 $e^{-4}$ \\
  4 & <United States President, livesIn, Washington, D.C> & 3.83 $e^{-4}$ \\
  5 & <United States President, politician, United States> & 3.31$e^{-4}$ \\
  6 & <Iraqi Army, isLocatedIn, Iraq> & 3.20$e^{-4}$ \\
  \hline
\end{tabular}
\label{iraq_pair-edge1}
\vspace{-1.5\baselineskip}
\end{table}

Table ~\ref{iraq_coll-node-attr} and Table ~\ref{iraq_coll-edge1} show the node attribute/node influence value and edge influence value of the collective comparative reasoning example we used in section ~\ref{exp-coll-section}.
\begin{table}[ht]
\vspace{-1\baselineskip}
\caption{Collective node attribute influence ranking}
\vspace{-1.0\baselineskip}
\scriptsize
\subfloat[Node attribute influence]
{\begin{tabular}{|c|c|c|}
\hline
\multicolumn{3}{|c|}{Node attribute influence: $KS_1$} \\
\hline
Rank & Predicate & value \\
\hline
1 & Washington,D.C & 2.93$e^{-5}$  \\
2 & White House & 2.71$e^{-5}$    \\
3 & United States & 1.59$e^{-5}$  \\
4 & United States President      & 1.47$e^{-5}$    \\
5 & Iraq &  1.47$e^{-5}$  \\
6 & Iraqi Army & 1.36$e^{-5}$    \\
\hline
\multicolumn{3}{|c|}{Node attribute influence: $KS_2$} \\
\hline
Rank & Predicate & value \\
\hline
1 & Washington,D.C   &   2.29 $e^{-4}$ \\
2 & White House      &   1.31 $e^{-4}$ \\
\hline
\multicolumn{3}{|c|}{Node attribute influence: $KS_3$} \\
\hline
Rank & Predicate & value \\
\hline
1 & Washington,D.C & 2.08 $e^{-4}$  \\
2 & United States President     & 1.10 $e^{-4}$   \\
3 & United States &  1.10$e^{-4}$  \\
4 & United States Army & 1.09$e^{-4}$    \\
5 & Operation  & 1.09$e^{-4}$ \\
~ & {Mountain Thrust} & ~\\
6 & Afghanistan & 1.09 $e^{-4}$    \\
\hline
\end{tabular}}
%\vspace*{-0cm}
\subfloat[Node influence]
{\begin{tabular}{|c|c|c|}
\hline
\multicolumn{3}{|c|}{Node influence: $KS_1$} \\
\hline
Rank & Predicate & value \\
\hline
1 & Washington,D.C & 4.57$e^{-6}$  \\
3 & United States & 3.57$e^{-6}$  \\
4 & United States President      & 2.35$e^{-6}$    \\
5 & Iraq &  2.26$e^{-6}$  \\
2 & White House & 2.17$e^{-6}$    \\
6 & Iraqi Army & 1.09$e^{-6}$    \\
\hline
\multicolumn{3}{|c|}{Node influence: $KS_2$} \\
\hline
Rank & Predicate & value \\
\hline
1 & Washington,D.C   &   7.68 $e^{-6}$ \\
2 & White House      &   7.68 $e^{-6}$ \\
\hline
\multicolumn{3}{|c|}{Node influence: $KS_3$} \\
\hline
Rank & Predicate & value \\
\hline
1 & Washington,D.C & 1.19 $e^{-5}$  \\
2 & United States President     & 1.19 $e^{-5}$   \\
3 & United States &  1.19$e^{-5}$  \\
4 & United States Army & 1.18$e^{-5}$    \\
5 & Operation & 1.18$e^{-5}$ \\
~ & {Mountain Thrust} & ~\\
6 & Afghanistan & 1.18 $e^{-5}$    \\
\hline
\end{tabular}}
\vspace{-1.5\baselineskip}
\label{iraq_coll-node-attr}
\end{table}
\begin{table}[ht]
\vspace{-1\baselineskip}
    \centering
    \caption{Collective edge influence ranking}
    \vspace{-1\baselineskip}
    \footnotesize
\begin{tabular}{ |c|c|c| }
  \hline
  \multicolumn{3}{|c|}{Edge influence of $KS_1$} \\
  \hline
  Rank & Triple & value \\
  \hline
  1 & <United States, hasCapital, Washington, D.C> & 1.20 $e^{-4}$ \\
  2 & <United States President, isPoliticianOf, United States> & 1.07 $e^{-4}$ \\
  3 & <United States President, livesIn, Washington, D.C> & 1.05 $e^{-4}$  \\
  4 & <United States, dealsWith, Iraq> &  9.94 $e^{-5}$ \\
  5 & <White House, isLocatedIn, Washington, D.C> & 8.22 $e^{-5}$ \\
  6 & <Iraqi Army, isLocatedIn, Iraq> & 6.47 $e^{-5}$ \\
  \hline
  \multicolumn{3}{|c|}{Edge influence of $KS_2$} \\
  \hline
    Rank & Triple & value \\
  \hline
  1 &  <White House, isLocatedIn, Washington, D.C> & 2.23 $e^{-4}$ \\
  \hline
  \multicolumn{3}{|c|}{Edge influence of $KS_3$} \\
  \hline
    Rank & Triple & value \\
  \hline
  1 & <United States President, livesIn, Washington, D.C> & 4.99$e^{-4}$ \\
  2 & <United States, hasCapital, Washington, D.C> & 4.99 $e^{-4}$ \\
  3 & <United States President, isLeaderOf, US Army> & 4.99 $e^{-4}$ \\
  4 & <United States, dealsWith, Afghanistan> &  4.99, $e^{-4}$ \\
  6 & <Afghanistan, participatedIn, Operation Mountain Thrust> & 4.99 $e^{-4}$ \\
  7 & <US Army, participatedIn, Operation Mountain Thrust> & 4.99$e^{-4}$ \\
  \hline
\end{tabular}
\label{iraq_coll-edge1}
\vspace{-1\baselineskip}
\end{table}

\FloatBarrier
\subsection{F -- Comparative Reasoning Examples}

\begin{figure}[ht]
	\centering
	\includegraphics[width=0.43\textwidth]{img/obama-honolulu.pdf}
	\caption{Pairwise consistency example.}
	\label{hawaii_honolulu}
	\vspace{-0.8\baselineskip}
\end{figure}

We give an additional example to evaluate the effectiveness of pairwise comparative reasoning. The query pair we used here is: <{\tt Barack Obama}, {\tt wasBornIn}, {\tt Hawaii}>, <{\tt Barack Obama}, {\tt wasBornIn}, {\tt Honolulu}>.

Figure ~\ref{hawaii_honolulu} shows the knowledge segments of <{\tt Barack Obama}, {\tt wasBornIn}, {\tt Hawaii}>, <{\tt Barack Obama}, {\tt wasBornIn}, {\tt Honolulu}> and <{\tt Honolulu}, {\tt isTypeOf}, {\tt Hawaii}>, respectively. 
We first check the consistency for <{\tt Barack Obama}, {\tt wasBornIn}, {\tt Hawaii}> and  <{\tt Barack Obama}, {\tt wasBornIn}, {\tt Honolulu}>. since the subject and predicates of these two clues are the same, we only need to check whether <{\tt Honolulu}, {\tt isTypeOf}, {\tt Hawaii}>. The predicate similarity between {\tt isTypeOf} and {\tt hasCapital} is 0.786 > 0.700. The information transfer amount between  {\tt Hawaii} and {\tt Honolulu}  is greater than 0.700 (i.e., \textrm{infTrans}({\tt Hawaii}, {\tt Honolulu}) > 0.700). This means this pair of clues are consistent with each other.

\hide{
Figure ~\ref{kenya-honolulu} shows the knowledge segments of <{\tt Barack Obama}, {\tt wasBornIn}, {\tt Kenya}>, <{\tt Barack Obama}, {\tt wasBornIn}, {\tt Honolulu}> and <{\tt Honolulu}, {\tt isTypeOf}, {\tt Kenya}>, respectively. The information transfer amount between {\tt Kenya} and {\tt Honolulu} calculated by our system is \textrm{infTrans}({\tt Kenya}, {\tt Honolulu}) = 0.569 < 0.700. This means that this pair of clues are inconsistent.
}

\hide{
Figure ~\ref{inconsistency-example} shows the corresponding knowledge segments of <{\tt Barack Obama}, {\tt refusedBy}, {\tt Air Force One}> and <{\tt Barack Obama}, {\tt inFrontOf}, {\tt Helicopter}>, extracted from the knowledge graph in Figure ~\ref{inconsistency}.
The node attribute influence value, node influence value, and edge influence value of $KS_1$ and $KS_2$ are shown
in Table ~\ref{pair-node-attr} and Table ~\ref{pair-edge1}
, respectively.
As we can see, 
for $KS_1$, the top-{\em 50\%} elements with the highest node attribute influence
are {\tt President}, {\tt US Army} and {\tt Barack Obama} which are the same as the top-{\em 50\%} elements with the highest node attribute influence in $KS_2$. 
For the top-{\em 50\%} elements with the highest node influence, $KS_1$ and $KS_2$ share the same elements, which are {\tt US Army}, {\tt President} and {\tt Air Force}.
As for the top-{\em 50\%} edges of $KS_1$ with the highest influence, there is one edge (<{\tt US Army}, {\tt command}, {\tt Air Force}>) which also belongs to the top-50\% edges of $KS_2$.
Therefore, the key elements overlapping rate between $KS_1$ and $KS_2$ is $\frac{1 + 1 + \frac{1}{3}}{3} = \frac{7}{9} > 60\%$. This means that these two clues refer to the same thing. 

We further check if there is any inconsistency between them. To this end, we extract the knowledge segment for <{\tt Helicopter}, {\tt isTypeOf}, {\tt Air Force One}> and <{\tt Air Force One}, {\tt isTypeOf}, {\tt Helicopter}>. 
The right hand side of Figure ~\ref{inconsistency-example} shows the knowledge segments for <{\tt Helicopter}, {\tt isTypeOf}, {\tt Air Force One}> (We obtain the same knowledge segment for <{\tt Air Force One}, {\tt isTypeOf}, {\tt Helicopter}>). 
The proposed TF-IDF predicate-predicate similarity between {\tt command} and {\tt isTypeOf} is $0.216$ . Based on that, we have \textrm{infTrans}({\tt Helicopter}, {\tt Air Force One}) = \textrm{infTrans}({\tt Air Force One}, {\tt Helicopter}) = $ 0.047 < 0.700$. This means that "Helicopter" and "Air Force One" are two different things. 
We get the same result for triple <{\tt Air Force One}, {\tt isTypeOf}, {\tt Helicopter}>. Therefore, we conclude that 
the two given clues are inconsistent. 

\begin{figure}[]
	\centering
	\includegraphics[width=0.35\textwidth]{img/exp_inconsistency.png}
	\caption{Example of pair-wise comparative reasoning.}
	\label{inconsistency-example}
	\vspace{-1\baselineskip}
\end{figure}
}

\hide{
\begin{table}[ht]
\caption{Pairwise Node Attribute/Node Influence Ranking}
\vspace{-0.5\baselineskip}
\small
\subfloat[Node Attribute Influence: $KS_1$]
{\begin{tabular}{|c|c|c|}
\hline
 Rank & Predicate & value \\
\hline
1 & President &  6.51 $e^{-5}$  \\
2 & US Army   &  6.35$e^{-5}$  \\
3 & Barack Obama & 6.02$e^{-5}$   \\
4 & Air Force & 5.87$e^{-5}$    \\
5 & Air Force One  & 3.15$e^{-5}$    \\
6 & 6000M & 2.82$e^{-5}$    \\
\hline
\end{tabular}}
%\vspace*{0.1cm}
\subfloat[Node Attribute Influence: $KS_2$]
{\begin{tabular}{|c|c|c|}
\hline
Rank & Predicate & value \\
\hline
1 & President &  6.52$e^{-5}$  \\
2 & US Army   &  6.35$e^{-5}$  \\
3 & Barack Obama & 6.03$e^{-5}$   \\
4 & Air Force & 5.87$e^{-5}$    \\
5 & Helicopter  & 3.15$e^{-5}$    \\
6 & 600M & 2.82$e^{-5}$    \\
\hline
\end{tabular}}
\\
\vspace{-1\baselineskip}
\subfloat[Node Influence: $KS_1$]
{\begin{tabular}{|c|c|c|}
\hline
Rank & Predicate & value \\
\hline
1 & US Army  & 1.91$e^{-5}$    \\
2 & President & 1.82$e^{-5}$    \\
3 & Air Force & 1.07 $e^{-5}$    \\
4 & Barack Obama &   9.85 $e^{-6}$  \\
5 & Air Force One & 8.67 $e^{-6}$    \\
6 & 6000M & 2.81$e^{-6}$  \\
\hline
\end{tabular}}
%\vspace*{2cm}
\subfloat[Node Influence: $KS_2$]
{\begin{tabular}{|c|c|c|}
\hline
Rank & Predicate & value \\
\hline
1 & US Army & 1.91$e^{-5}$     \\
2 & President  & 1.82$e^{-5}$      \\
3 & Air Force    &   1.07$e^{-5}$      \\
4 & Barack Obama    &   9.85$e^{-6}$      \\
5 & Helicopter      &   8.67$e^{-6}$ \\
6 & 600M   &   2.82$e^{-6}$ \\
\hline
\end{tabular}}
\label{pair-node-attr}
\vspace{-2\baselineskip}
\end{table}

\begin{table}[ht]
    \centering
    \small
    \caption{Pairwise Edge influence Ranking}
    \vspace{-0.5\baselineskip}
    \begin{tabular}{ |c|c|c| }
\hline
\multicolumn{3}{|c|}{Edge Influence of $KS_1$} \\\hline
  Rank & Triple & value \\
  \hline
  1 & <US Army, command, Air Force One> & 8.14 $e^{-4}$ \\
  2 & <Air Force, command, Air Force One> & 7.14 $e^{-4}$ \\
  3 & <US Army, command, Air Force> & 7.13$e^{-4}$ \\
  4 & <President, inCharge, US Army> & 6.99$e^{-4}$ \\
  5 & <Air Force One, maximumDistance, 6000M> & 5.88$e^{-4}$ \\
  6 & <Barack Obama, nominate, President> & 4.94$e^{-4}$ \\
  \hline
  \multicolumn{3}{|c|}{Edge Influence of $KS_2$} \\\hline
  Rank & Triple & value \\
  \hline
  1 & <US Army, command, Helicopter> & 8.14$e^{-4}$ \\
  2 & <Air Force, command, Helicopter> & 7.13$e^{-4}$ \\
  3 & <US Army, command, Air Force> & 7.00$e^{-4}$ \\
  4 & <President, inCharge, US Army> & 6.99$e^{-4}$ \\
  5 & <Helicopter, maximumDistance, 6000M> & 5.89$e^{-4}$ \\
  6 & <Barack Obama, nominate, President> & 4.93$e^{-4}$ \\
  \hline
\end{tabular}
\label{pair-edge1}
\vspace{-2\baselineskip}
\end{table}

}

\subsection{G -- Collective Comparative Reasoning Examples}

\begin{figure}[]
\vspace{-1\baselineskip}
	\centering
	\includegraphics[width=0.44\textwidth, height=0.26\textwidth]{img/obama-coll.pdf}
	\vspace{-1\baselineskip}
	\caption{Example of collective comparative reasoning.}
	\label{exp-coll}
	\vspace{-1\baselineskip}
\end{figure}

Here we give another collective comparative reasoning example. The query graph we used is:  <{\tt Barack Obama}, {\tt refusedBy}, {\tt Air Force One}>, <{\tt President}, {\tt inFrontOf}, {\tt Helicopter}>, <{\tt Barack Obama}, {\tt is}, {\tt President}>.
Figure ~\ref{exp-coll} shows the query graph and the corresponding semantic matching subgraph. 
If we check each pair of clues in the query graph, we find that the key elements overlapping rate between $KS_1$ and $KS_3$ is more than 60\%. This is because the overlapping rates  are $100\%$ for node attribute influence, $50\%$ for node influence and $50\%$ for edge influence, which give the average overlapping rate $\frac{1 + \frac{1}{2} + \frac{1}{2}}{3} = \frac{2}{3} > 60\%$.

Based on this, we future check <{\tt Barack Obama}, {\tt isTypeOf}, {\tt President}> or <{\tt President}, {\tt isTypeOf}, {\tt Barack Obama}>. Our TF-IDF based predicate-predicate similarity between "{\tt isTypeOf}" and "{\tt is}" is 1.00. Thus, we have \textrm{infTrans}({\tt Barack Obama}, {\tt President}) $= 1.00 > 0.700$. This means that these two knowledge segments have the same subject. Finally, we check  <{\tt Helicopter}, {\tt isTypeOf}, {\tt Air Force One}> or <{\tt Air Force One}, {\tt isTypeOf}, {\tt Helicopter}>. The right part of Figure ~\ref{exp-coll} shows the corresponding knowledge segment. The proposed TF-IDF predicate-predicate similarity between {\tt command} and {\tt isTypeOf} is $0.216$ . Based on that, we have \textrm{infTrans}({\tt Helicopter}, {\tt Air Force One}) = \textrm{infTrans}({\tt Air Force One}, {\tt Helicopter}) = $ 0.047 < 0.700$. This means that "Helicopter" and "Air Force One" are two different things.  
Therefore, we conclude that this query graph is inconsistent.

\begin{table}[]
\caption{Collective Node Attribute Influence Ranking}
\vspace{-1\baselineskip}
\scriptsize
\subfloat[Node Attribute Influence]
{\begin{tabular}{|c|c|c|}
\hline
\multicolumn{3}{|c|}{Node Attribute Influence: $KS_1$} \\
\hline
Rank & Predicate & value \\
\hline
1 & President      & 3.53$e^{-4}$    \\
2 & US Army & 2.12$e^{-4}$    \\
3 & Helicopter & 2.09$e^{-4}$    \\
4 & Air Force &  1.91$e^{-4}$  \\
5 & 600M & 1.78$e^{-4}$  \\
\hline
\multicolumn{3}{|c|}{Node Attribute Influence: $KS_2$} \\
\hline
Rank & Predicate & value \\
\hline
1 & President      &   6.54$e^{-4}$ \\
2 & Barack Obama   &   4.81$e^{-4}$ \\
\hline
\multicolumn{3}{|c|}{Node Attribute Influence: $KS_3$} \\
\hline
Rank & Predicate & value \\
\hline
1 & President     & 3.24$e^{-4}$    \\
2 &  Barack Obama & 3.13$e^{-4}$ \\
3 & US Army & 1.81$e^{-4}$    \\
4 & Air Force One & 1.79$e^{-4}$    \\
5 & Air Force &  1.73$e^{-4}$  \\
6 & 6000M & 1.51$e^{-4}$  \\
\hline
\end{tabular}}
%\vspace*{-0cm}
\subfloat[Node Influence]
{\begin{tabular}{|c|c|c|}
\hline
\multicolumn{3}{|c|}{Node Influence: $KS_1$} \\
\hline
Rank & Predicate & value \\
\hline
1 & US Army      & 4.74$e^{-5}$    \\
2 & Helicopter & 4.73 $e^{-5}$   \\
3 & Air Force & 3.16  $e^{-5}$  \\
4 & President &  1.52 $e^{-5}$  \\
5 & 600M & 1.52 $e^{-5}$  \\
\hline
\multicolumn{3}{|c|}{Node Influence: $KS_2$} \\
\hline
Rank & Predicate & value \\
\hline
1 & Barack Obama   &   3.75$e^{-5}$ \\
2 & President      &   3.75$e^{-5}$ \\
\hline
\multicolumn{3}{|c|}{Node Influence: $KS_3$} \\
\hline
Rank & Predicate & value \\
\hline
1 & US Army     &  4.03$e^{-5}$    \\
2 &  Air Force One & 3.98$e^{-5}$ \\
3 & President & 3.73$e^{-5}$    \\
4 & Air Force & 2.66$e^{-5}$    \\
5 & Barack Obama &  2.40$e^{-5}$  \\
6 & 6000M & 1.28$e^{-5}$  \\
\hline
\end{tabular}}
\label{coll-node-attr1212}
\end{table}

\begin{table}[]
    \centering
    \caption{Collective Edge Influence Ranking of KS1}
    \vspace{-1\baselineskip}
    \scriptsize
\begin{tabular}{ |c|c|c| }
  \hline
  \multicolumn{3}{|c|}{Edge Influence of $KS_1$} \\
  \hline
  Rank & Triple & value \\
  \hline
  1 & <US Army, command, Helicopter> & 1.64$e^{-3}$ \\
  2 & <US Army, command, Air Force> & 1.42$e^{-3}$ \\
  3 & <Air Force, command, Helicopter> & 1.38$e^{-3}$ \\
  4 & <President, inCharge, US Army> & 1.10 $e^{-3}$\\
  5 & <Helicopter, maximumDistance, 600M> & 1.10$e^{-3}$ \\
  \hline
  \multicolumn{3}{|c|}{Edge Influence of $KS_2$} \\
  \hline
    Rank & Triple & value \\
  \hline
  1 & <Barack Obama, nominate, President> & 3.75 $e^{-5}$ \\
  \hline
  \multicolumn{3}{|c|}{Edge Influence of $KS_3$} \\
  \hline
    Rank & Triple & value \\
  \hline
  1 & <US Army, command, Air Force One> & 1.31$e^{-3}$ \\
  2 & <US Army, command, Air Force> & 1.21$e^{-3}$ \\
  3 & <Air Force, command, Air Force One> & 1.18$e^{-3}$ \\
  4 & <President, inCharge, US Army> & 1.10$e^{-3}$ \\
  5 & <Air Force One, maximumDistance, 6000M> & 9.32$e^{-4}$ \\
  6 & <Barack Obama, nominate, President> & 7.27 $e^{-4}$\\
  \hline
\end{tabular}
\label{coll-edge1212}
\end{table}

\hide{
\begin{table}[]
    \centering
    \caption{Predicate Similarity of {\tt isTypeOf} with others}
    \begin{tabular}{ |l|l|c| }
  \hline
  predicate & predicate & similarity \\
  \hline
isTypeOf &  isLeaderOf &  0.955 \\
isTypeOf &  owns &  0.945\\
isTypeOf &  isTypeOf &  1.000\\
isTypeOf &  isLocatedIn &  0.870\\
isTypeOf &  ark Architects &  0.000\\
isTypeOf &  hasMusicalRole &  0.688\\
isTypeOf &  hasOfficialLanguage &  0.697\\
isTypeOf &  edited &  0.638\\
isTypeOf &  isConnectedTo &  0.603\\
isTypeOf &  actedIn &  0.725\\
isTypeOf &  imports &  0.693\\
isTypeOf &  participatedIn &  0.869\\
isTypeOf &  wasBornIn &  0.989\\
isTypeOf &  dealsWith &  0.697\\
isTypeOf &  created &  0.700\\
isTypeOf &  diedIn &  0.785\\
isTypeOf &  isPoliticianOf &  0.917\\
isTypeOf &  wroteMusicFor &  0.762\\
isTypeOf &  hasNeighbor &  0.686\\
isTypeOf &  isMarriedTo &  0.815\\
isTypeOf &  hasChild &  0.807\\
isTypeOf &  isInterestedIn &  0.802\\
isTypeOf &  isAffiliatedTo &  0.808\\
isTypeOf &  hasCurrency &  0.697\\
isTypeOf &  exports &  0.706\\
isTypeOf &  happenedIn &  0.767\\
isTypeOf &  hasGender &  0.840\\
isTypeOf &  playsFor &  0.812\\
isTypeOf &  directed &  0.754\\
isTypeOf &  worksAt &  0.752\\
isTypeOf &  graduatedFrom &  0.822\\
isTypeOf &  hasCapital &  0.786\\
isTypeOf &  influences &  0.804\\
isTypeOf &  hasWonPrize &  0.889\\
isTypeOf &  hasWebsite &  0.912\\
isTypeOf &  rown &  0.000\\
isTypeOf &  livesIn &  0.972\\
isTypeOf &  hasAcademicAdvisor &  0.745\\
isTypeOf &  isKnownFor &  0.760\\
isTypeOf & isCitizenOf &  0.840 \\
  \hline
\end{tabular}
    
\label{appendix-pred-sim}
\end{table}
}

\hide{
\subsection{C -- Relevant Entities Query}

Besides the functions we described above, \gchecker\ also supports {\em top-}10 most relevant entities searching. More specifically speaking, given a query entity,  \gchecker\ will find the most similar 10 entities w.r.t. the query entity in the knowledge graph.
Table ~\ref{similar-nodes} shows the most similar entities in the knowledge graph w.r.t the query entity by knowledge embedding and entropy based random walk with restart, respectively. As we can see the entities found by Entropy Random walk with restart have a very high quality. These entities can directly give us a lot of information about "Barack Obama". When we see these results, we can easily know that Barack Obama is a male who is an United states citizen. And he is a politician who belongs to Democratic party. He has a strong connection with two cities, Honolulu and Chicago, and a person who named Michelle Obama.

\begin{table}[ht]
    \centering
    \caption{Top 10 similar entities of Barack Obama}
    
    \begin{tabular}{ |l|l|c| }
  \hline
  Ranking & Entropy Random walk with Restart& TransE \\
  \hline
  1 & United States & A \\
  2 & Washington, D.C & B \\
  3 & United States dollar & B \\
  4 & Honolulu & C \\
  5 & http://www.dc.gov & D \\
  6 & Chicago & E \\
  7 & North America & E \\
  8 & male & E \\
  9 & Democratic Party & E \\
  10 & Michelle Obama & E \\
  \hline
\end{tabular}
    
\label{similar-nodes}
\end{table}
}
